# Supplementary material for: LINC: A Neurosymbolic Approach for Logical Reasoning by Combining Language Models with First-Order Logic Provers
Source: arXiv:2310.15164 source file (2024-02-14)
Supplement: Supplementary file 1 [file appendix_logic_lm.tex]

\section{Detailed comparison with \citet{pan2023logic}} \label{sec:appendix-logiclm}
Concurrently, as we were wrapping up this work, \citet{pan2023logic} released Logic-LM, a neurosymbolic framework for logical reasoning that shares many high-level similarities with our framework.
Overall, our work focuses more on understanding the relative benefits and drawbacks of neurosymbolic reasoning approaches compared to traditional in-context reasoning approaches like \texttt{Chain-of-Thought}, which we highlight through our detailed error analysis.

In terms of the framework and algorithmic components themselves, we identify a few key differences\footnote{Throughout this section, Logic-LM refers to the version on \url{https://arxiv.org/abs/2305.12295}, which is the latest version at the time of writing}: 
\begin{itemize}
    \item Algorithmically, Logic-LM applies an additional self-refine step to boost their performance and conducts a detailed ablation on its impact. We believe these insights could help improve the results of our neurosymbolic method as well.
    \item While Logic-LM only considers one prediction, we sample many predictions and employ a majority voting scheme, which has been found to be beneficial in reasoning domains \citep{wang2022self}. See Appendix~\ref{appendix:k_way} for a brief discussion of the impact this has on performance in \texttt{LINC}.
    \item On FOLIO, we use a filtered version of the validation set with 22 less samples (see Appendix \ref{appendix_folio_dataset}). On ProofWriter, we evaluate on substantially a smaller subset (360 vs. 600 samples); however, we ensure that this subset is not only balanced across the classes but also across the deductive depth required, something which the authors of Logic-LM do not mention doing. Additionally, we take great care to make sure that the labels are even uniformly distributed \emph{within} each depth subset, to make sure that our results in Figure~\ref{fig:results-qdep} are not biased. Finally, since Logic-LM puts a greater focus on breadth in their evaluation, they evaluate on two additional datasets (PrOntoQA and LogicalDeduction); meanwhile, we focus here on in-depth error analysis for FOLIO and ProofWriter exclusively.
    \item On our ProofWriter evaluation, we evaluate an out-of-distribution setting by using few-shot examples from the FOLIO dataset, while Logic-LM uses in-distribution few-shot examples from ProofWriter (likely handwritten, as these do not come with the dataset)\footnote{Based on \href{https://github.com/teacherpeterpan/Logic-LLM/blob/3c13afd0cb9f4a7391ebe2609ef9330e743f0965/models/prompt_library.py}{their latest code at the time of writing}}.
    \item We use a different FOL representation than Logic-LM. We hypothesize that our FOL representation is both simpler and more similar to natural language, which should benefit language models trained on large amounts of text.
    \item In terms of models, we include the open-access model StarCoder+, and our primary focus is on StarCoder+ and GPT-3.5 (due to the cost constraint of GPT-4). On the other hand, Logic-LM performs their evaluation with GPT-3.5 and GPT-4, highlighting a more thorough analysis with GPT-4 but sacrificing a comparison to an open-access model.
    \item While our raw numbers are not directly comparable due to the dataset differences mentioned above, we find some high-level differences in trends. First, we notice a larger gap between \texttt{CoT} and the neurosymbolic approach (\texttt{LINC} in our case; Logic-LM in theirs) on the ProofWriter dataset. This may be because our FOL representation is more concise, making the NL to FOL translation task easier for the LM. Second, we find that with GPT-4, chain-of-thought prompting performs as good as our neurosymbolic method. This may be because we use an updated version of GPT-4 (gpt-4-0613), which was not released at the time the Logic-LM preprint was last updated. 
\end{itemize}
